# Supplementary material for: Pressure control using stochastic cell rescaling
Source: arXiv:2006.09250 ancillary file (2020-08-26)
Supplement: Supplementary file 1 [file si.pdf]

# Supplementary Material: Pressure control using stochastic cell rescaling

Mattia Bernetti[1] and Giovanni Bussi[1, a)]

*Scuola Internazionale Superiore di Studi Avanzati, Via Bonomea 265, Trieste 34136, Italy*

(Dated: 25 August 2020)

[a)]Electronic mail: bussi@sissa.it

# Part I

# Supplementary Methods

## I. CENTER OF MASS CONTRIBUTION TO THE PRESSURE

For a system where the potential energy is invariant with respect to rigid translations, the total momentum is conserved. This conservation can be broken for instance by the presence of a local thermostat, such as the Langevin thermostat. If using such a thermostat, the kinetic contribution to the internal pressure will be equal, on average, to $\frac{Nk_BT}{V}$, where $N$ is the number of atoms. However, if a global thermostat is used and the initial momentum of the center of mass is set to zero, then its motion will be decoupled from that of the other particles. As a consequence, the kinetic contribution to the internal pressure will be equal, on average, to $\frac{(N-1)k_BT}{V}$. It is possible to add a correction so as to make the results obtained with local and global thermostats identical. Indeed, one might argue that, as soon as the transfer of energy and mechanical work to an external reservoir is allowed, also the center-of-mass motion should be coupled with the thermal bath. By rewriting the $NPT$ ensemble in coordinates relative to the center of mass, one obtains

$$\mathscr{P}(p,q,V) \propto Ve^{-\frac{K+U+P_0V}{k_BT}} \delta\left(\sum_i m_i \boldsymbol{q}_i\right) \delta\left(\sum_i \boldsymbol{p}_i\right) . \tag{S1}$$

The extra $V$ term originates from the integration of the center of mass coordinate and contributes to the internal pressure. The effect of including this term is simply an additional contribution to the internal pressure:

$$P'_{\text{int}} = P_{\text{int}} + \frac{k_BT}{V} \tag{S2}$$

In the main text, we describe two alternative ways to compute the internal pressure, namely (a) from the instantaneous kinetic energy or (b) from the average kinetic energy. In the first formulation, the term above corresponds to adding to the average kinetic energy the contribution of the center of mass, $\frac{3}{2}k_BT$. We remark that one should add the *average* kinetic energy rather than the istantaneous one, since the rescaling operation is not affecting the center-of-mass momentum that, in the reference system of the simulation, is zero. In the second formulation, the term above corresponds to computing the kinetic contribution to the internal pressure as $\frac{Nk_BT}{V}$ where $N$ is the number of atoms, *without* subtracting 1 as suggested in the main text.

We notice that the contribution of the center of mass to the internal pressure was also included for instance in Ref. 1. Other algorithms, instead, such as the one in Ref. 2, did not include this contribution. We also notice that there is some ambiguity in the definition of the $NPT$ ensemble in the literature. For instance, if one uses the logarithm of the volume as the integration variable as suggested by Attard,[3] an additional $V^{-1}$ term should be included in the $NPT$ distribution. This term would cancel exactly the extra $V$ term in Eq. S1.

We decided *not* to include the contribution of the center of mass pressure in the simulations presented in this work, in order to have a definition for the $NPT$ ensemble that is coherent with the majority of the literature. As a consequence, internal pressure was computed either using the kinetic energy ($\frac{2K}{3V}$) or using its average value ($\frac{Nk_BT}{V}$ where $N$ is the number of atoms minus one if the center of mass momentum is zero). If desired, the contribution can be straightforwardly included by adding $\frac{k_BT}{V}$ to the definition of the internal pressure (as in Eq. S2). If one were using a local thermostat (such as the Langevin thermostat) or two separate global thermostats adding up to the entire system (*e.g.*, one global thermostat on the solute and one on the solvent), then no extra term would be required, since the instantaneous kinetic energy $K$ would already include the center-of-mass contribution, and its average value would be proportional to the number of atoms $N$. In the membrane simulations reported in this paper, thus, the center-of-mass contribution to the pressure is implicitly included by the usage of two reference groups for temperature coupling, and not included in the other simulations. We stress that the contribution of this term to the internal pressure is in practice negligible for systems with more than a hundred particles.

## II. EQUIVALENCE WITH LANGEVIN PISTON

We here show how Eq. 5 can be obtained as a limiting case of a Langevin piston thermostat for high friction. We first notice that the Langevin piston was initially[4] introduced on top of the Andersen barostat.[5] However, a Langevin thermostat on the auxiliary variable can be applied on top of any second-order barostat. For instance, in Ref. 6, a Langevin thermostat was applied on the auxiliary variable of a Martyna-Tobias-Klein barostat.[2] The difference between different second-order barostats is expected to be negligible when the number of simulated particles is large.

We will here start with a Langevin piston obtained by applying a Langevin thermostat on the

auxiliary variable of the barostat introduced in Ref. 1:

$$\dot{\eta} = \frac{3\left[V\left(P_{\rm int} - P_0\right) + k_B T\right]}{W} - \gamma(V)\eta + \sqrt{\frac{2k_B T \gamma(V)}{W}}\xi(t) \tag{S3a}$$

$$\dot{\varepsilon} = 3\eta \tag{S3b}$$

Here $W$ is the mass associated to the piston and $\varepsilon = \log(V/V_0)$ is the strain. When compared with the barostat presented in Ref. 1, Eq. S3a contains an additional noise and friction term, controlled by a coefficient $\gamma$. This coefficient is explicitly written as a function of the volume $V$ for reasons that will be clear below. We also notice that Eq. S3a does not include the center of mass contribution to the pressure (see Section I) that might be optionally included as an additional $\frac{k_B T}{V}$ contribution to $P_{\rm int}$ in order to recover the ensemble discussed in Ref. 1.

Equation S3a can be rewritten as a second-order differential equation:

$$W\ddot{\varepsilon} = 9\left[V\left(P_{\rm int} - P_0\right) + k_B T\right] - \gamma(V)W\dot{\varepsilon} + \sqrt{18 k_B T \gamma(V) W}\xi(t) \tag{S4}$$

Taking the high-friction limit of this equation, where $\gamma$ diverges but $\gamma W$ is finite, is not trivial since the explicit dependence of $\gamma$ on $V$ (and thus on $\varepsilon = \log(V/V_0)$) leads to an additional drift term.[7] After taking the limit as in Eq. 97 of Ref. 7, the resulting equation for $\varepsilon$ is

$$d\varepsilon = \left(\frac{9\left[V\left(P_{\rm int} - P_0\right) + k_B T\right]}{W\gamma(V)} - \frac{9k_B T}{W\gamma(V)}\frac{1}{\gamma}\frac{d\gamma}{d\varepsilon}\right)dt + \sqrt{\frac{18 k_B T W}{\gamma(V)}}dW \tag{S5}$$

We now arbitrarily set $\gamma(V) = \frac{9\tau_P V}{W\beta_T}$. The drift term is then proportional to $\frac{1}{\gamma}\frac{d\gamma}{d\varepsilon} = \frac{1}{\gamma}\frac{d\gamma}{dV}\frac{dV}{d\varepsilon} = 1$. After substitution, the drift term cancels exactly the $k_B T$ term. One thus obtains Eq. 5.

The specific choice of $\gamma(V)$ is arbitrary, similarly to the choice of $D$ in the main text. The reason for our choice is to obtain a first-order equation where the deterministic part is identical to the one used in the Berendsen barostat.

In summary, the stochastic cell rescaling barostat can be seen as the barostat of Ref. 1 plus a Langevin thermostat applied to the barostat degree of freedom, provided that the limit of large friction and zero mass is taken, and that one sets $W\gamma = \frac{9\tau_P V}{\beta_T}$.

## III. PROPAGATING THE BAROSTAT EQUATION

We here discuss how to propagate the dynamics of $\varepsilon = \log(V/V_0)$ in order to minimize detailed balance violations. The simplest possible way to propagate $\varepsilon$ is by finite difference:

$$\varepsilon(t+\Delta t) = \varepsilon(t) - \frac{\beta_T}{\tau_P}\left(P_0 - P_{\rm int}(t)\right)\Delta t + \sqrt{\frac{2k_B T \beta_T}{V_0 e^{\varepsilon(t)}\tau_P}\Delta t}R(t) \tag{S6}$$

where $R(t)$ is a Gaussian random number with zero average and unitary variance. In order to compute the drift in the effective energy associated to this move it is necessary to compute the ratio between the probability of generating this move and the probability of generating the opposite move.[8] In the limit of small $\Delta t$ or, equivalently, large $\tau_P$, the transition probability is dominated by the stochastic term. In order to maximize the chance to generate the opposite move, it is convenient that the variance of the noise is independent of the evolved variable. This can be obtained by means of a change of variable $\lambda = e^{\varepsilon/2}\sqrt{V_0}$ (see Eq. 7). The propagation of $\lambda$ is then given by

$$\lambda(t+\Delta t) = \lambda(t) - \frac{\beta_T \lambda(t)}{2\tau_P}\left(P_0 - P_{\text{int}}(t) - \frac{k_B T}{2\lambda^2(t)}\right)\Delta t + \sqrt{\frac{k_B T \beta_T}{2\tau_P}\Delta t} R(t) \ . \tag{S7}$$

## IV. COMPUTING THE EFFECTIVE ENERGY DRIFT

The stationary distribution for $\lambda$ at fixed scaled coordinates is:

$$\mathscr{P}(\lambda) \propto e^{-\frac{K+U+P_0\lambda^2}{k_B T}} \lambda \tag{S8}$$

where the extra $\lambda \propto \frac{dV}{d\lambda}$ originates from the change of variable. This is equivalently written as

$$-k_B T \log \mathscr{P}(\lambda) = K + U + P_0\lambda^2 - k_B T \log \lambda + C \tag{S9}$$

where $C$ is an arbitrary constant. By defining $D = \frac{k_B T \beta_T}{4\tau_P}$ as the diffusion constant for $\lambda$ and $f = -2\lambda\left(P_0 - P_{\text{int}} - \frac{k_B T}{2\lambda^2}\right)$ we can rewrite the dynamics of $\lambda$ (Eq. S7) as

$$\lambda(t+\Delta t) = \lambda(t) + \frac{D}{k_B T} f(\lambda)\Delta t + \sqrt{2D} R(t) \tag{S10}$$

This form is identical to the high friction Langevin equation discussed in the Appendix of Ref. 8. The increment in effective energy is thus equal to

$$\Delta\tilde{H} = \Delta K + \Delta U + P_0\Delta\lambda^2 - k_B T \Delta \log \lambda + \Delta\lambda\left(\frac{f(\lambda(t)) + f(\lambda(t+\Delta t))}{2}\right) + \frac{\beta_T \Delta t}{4\tau_P k_B T}\Delta(f^2) \ . \tag{S11}$$

The last term results in a fluctuation, whereas the first four terms approximately cancel with the sum of the increments originating from the fifth term. This imperfect cancellation gives rise to a steady drift of the effective energy.

When using the formulation where momenta are not scaled when volume changes, $K$ will not change when applying the barostat but a term $-k_B T N \Delta \log V = -2 k_B T N \Delta \log \lambda$ should be added instead.

When including the contribution of the center-of-mass motion to the internal pressure (see Section I of these Supplementary Methods), one should add a further contribution equal to $-k_B T \Delta \log V = -2 k_B T \Delta \log \lambda$.

## V. FINITE TIME-STEP INTEGRATORS

We here derive the finite time-step integrators tested in this work. All of them are assumed to be combined with a velocity Verlet algorithm and a thermostat with a reversible scheme similar to the one introduced in Ref. 8, where the thermostat is applied in two steps, before and after the propagation of the Hamilton equations. In all of them, one can use either the kinetic energy or its average value to compute the internal pressure, as commented.

### A. Euler

1. Evolve thermostat for half a step.
2. If step is a multiple of $N_P$, use internal pressure to propagate volume and scale positions accordingly. If internal pressure was computed using the instantaneous kinetic energy, scale velocities with an inverse factor.
3. Act with forces on velocities for half a step. Forces are those obtained *before* volume scaling.
4. Act with velocities on positions.
5. Update forces based on current positions.
6. Act with forces on velocities for half a step.
7. Evolve thermostat for half a step.

This integrator is not reversible, since forces are not recomputed after volume scaling. As a consequence, the effective energy drift cannot be computed. Notice that we apply the barostat after the first evolution of the thermostat. This further breaks reversibility, and is done here so as to test the results in a case where the thermostat is applied in a single operation at the end of the time step, since this is commonly done in codes based on the leap-frog variant of velocity Verlet.

## B. Reversible

1. If step is a multiple of $N_P$, use internal pressure to propagate volume and scale positions accordingly. If internal pressure was computed using the instantaneous kinetic energy, scale velocities with an inverse factor.

2. Update forces based on current positions.

3. Evolve thermostat for half a step.

4. Act with forces on velocities for half a step.

5. Act with velocities on positions.

6. Update forces based on current positions.

7. Act with forces on velocities for half a step.

8. Evolve thermostat for half a step.

This algorithm resembles the Monte Carlo barostat[9,10] in the fact that, at the step when the volume is changed, an additional calculation of energy (or, in this case, forces) is required. The algorithm is reversible, and the effective energy drift can be computed.

## C. Trotter

1. Evolve thermostat for half a step.

2. Act with forces on velocities for half a step.

3. If step is a multiple of $N_P$, use internal pressure to propagate volume.

4. If step is a multiple of $N_P$, act with velocities on positions and simultaneously update volume and scale positions accordingly. Otherwise, act with velocities on positions.

5. Update forces based on current positions.

6. Act with forces on velocities for half a step.

7. Evolve thermostat for half a step.

Step number 4 should be implemented so that the Jacobian of the transformation is exactly equal to $(V'/V)^N$, where $V$ and $V'$ are the values of the volume before and after the scaling. A possible way to implement this step is to use a further Trotter splitting, where velocities are used to propagate positions for half a step, then positions (and, optionally, velocities) are scaled, then velocities are used to propagate positions for the remaining half step. Depending on which formulation of the algorithm one adopts, there are two different implementations:

- *Velocities are scaled.* This is the implementation used when the internal pressure is computed using the instantaneous kinetic energy. The propagation reads

$$q_i(t+\Delta t/2) = q_i(t) + \frac{p_i(t+\Delta t/2)}{m_i}\Delta t/2 \tag{S12a}$$

$$p_i^\star(t+\Delta t/2) = p_i(t+\Delta t/2)\sqrt[3]{\frac{V}{V'}} \tag{S12b}$$

$$q_i^\star(t+\Delta t/2) = q_i(t+\Delta t/2)\sqrt[3]{\frac{V'}{V}} \tag{S12c}$$

$$q_i(t+\Delta t) = q_i^\star(t+\Delta t/2) + \frac{p_i^\star(t+\Delta t/2)}{m_i}\Delta t/2 \tag{S12d}$$

  This can be equivalently written as

$$q_i(t+\Delta t) = q_i(t) + \left(\sqrt[3]{\frac{V}{V'}} + \sqrt[3]{\frac{V'}{V}}\right)\frac{p_i(t+\Delta t/2)}{m_i}\Delta t \tag{S13a}$$

$$p_i^\star(t+\Delta t/2) = p_i(t+\Delta t/2)\sqrt[3]{\frac{V}{V'}} \tag{S13b}$$

- *Velocities are not scaled.* This is the implementation used when the internal pressure is computed using the average kinetic energy. The propagation reads

$$q_i(t+\Delta t/2) = q_i(t) + \frac{p_i(t+\Delta t/2)}{m_i}\Delta t/2 \tag{S14a}$$

$$q_i^\star(t+\Delta t/2) = q_i(t+\Delta t/2)\sqrt[3]{\frac{V'}{V}} \tag{S14b}$$

$$q_i(t+\Delta t) = q_i^\star(t+\Delta t/2) + \frac{p_i(t+\Delta t/2)}{m_i}\Delta t/2 \tag{S14c}$$

  This can be equivalently written as

$$q_i(t+\Delta t) = q_i(t) + \left(1 + \sqrt[3]{\frac{V'}{V}}\right)\frac{p_i(t+\Delta t/2)}{m_i}\Delta t \tag{S15}$$

By evolving velocities, positions, and volume simultaneously, one does not need the additional force calculation that is needed in the Reversible implementation, still preserving time reversibility. However, in order to compute the effective energy drift, it is necessary to recompute the virial also at the step after the one in which volume was scaled.

## VI. EQUATIONS FOR THE SEMI-ISOTROPIC VERSION

In order to sample the constant surface tension ensemble, $\mathscr{P}(p,q,A,L) \propto e^{-\frac{K+U+P_0AL-\gamma_0 A}{k_BT}}$, it is necessary to write first the dynamics of the $A$ and $L$ variables. Using the same approach described in the main text, we obtain the following equations:

$$dA = D_A \frac{\partial \log(D_A \mathscr{P})}{\partial A} dt + \sqrt{2D_A} dW_A \tag{S16a}$$

$$dL = D_L \frac{\partial \log(D_L \mathscr{P})}{\partial L} dt + \sqrt{2D_L} dW_L \ . \tag{S16b}$$

We then set arbitrarily $D_A = \frac{2\beta_T A^2 k_B T}{3V\tau_P} = \frac{2\beta_T A k_B T}{3L\tau_P}$ and $D_L = \frac{\beta_T L^2 k_B T}{3V\tau_P} = \frac{\beta_T L k_B T}{3A\tau_P}$, and substitute the stationary distribution $\mathscr{P}$ defined in Eq. 8, obtaining:

$$dA = -\frac{2\beta_T}{3\tau_P}\frac{A}{L}\left(P_0 L - \gamma_0 + \frac{\partial K}{\partial A} + \frac{\partial U}{\partial A} - \frac{k_B T}{A}\right) dt + \sqrt{\frac{4\beta_T A^2 k_B T}{3V\tau_P}} dW_A \tag{S17a}$$

$$dL = -\frac{\beta_T}{3\tau_P}\frac{L}{A}\left(\frac{\partial K}{\partial L} + \frac{\partial U}{\partial L} - \frac{k_B T}{L}\right) dt + \sqrt{\frac{2\beta_T L^2 k_B T}{3V\tau_P}} dW_L \ . \tag{S17b}$$

After the change of variable $\varepsilon_{xy} = \log(A/A_0)$ and $\varepsilon_z = \log(L/L_0)$, by using the Ito chain rule we obtain the following equations of motion

$$d\varepsilon_{xy} = -\frac{2\beta_T}{3\tau_P}\frac{1}{L}\left(P_0 L - \gamma_0 + \frac{\partial K}{\partial A} + \frac{\partial U}{\partial A}\right) dt + \sqrt{\frac{4\beta_T k_B T}{3V\tau_P}} dW_{xy} \tag{S18a}$$

$$d\varepsilon_z = -\frac{\beta_T}{3\tau_P}\frac{1}{A}\left(\frac{\partial K}{\partial L} + \frac{\partial U}{\partial L}\right) dt + \sqrt{\frac{2\beta_T k_B T}{3V\tau_P}} dW_z \ . \tag{S18b}$$

We now exploit the following relationships between derivatives of the energy terms and the components of the pressure tensor:

$$\frac{P_{\mathrm{int},xx} + P_{\mathrm{int},yy}}{2} = \frac{1}{L}\left(\frac{\partial K}{\partial A} + \frac{\partial U}{\partial A}\right) \tag{S19a}$$

$$P_{\mathrm{int},zz} = \frac{1}{A}\left(\frac{\partial K}{\partial L} + \frac{\partial U}{\partial L}\right) \tag{S19b}$$

By replacing these relationships in Eqs. S18 we obtain the dynamics for $\varepsilon_{xy}$ and $\varepsilon_z$ of Eq. 9.

## VII. CONSTRAINING THE CELL HEIGHT

It is possible to set $D_L = 0$ in Eqs. S16 so as to obtain a semi-isotropic implementation where the cell height is frozen. This might be useful, *e.g.*, to simulate a membrane surrounded by an empty region. In this case, the dynamics of the $\varepsilon_{xy}$ will be given by Eq. 9a. Notice that this equation apparently contains an explicit dependence on $L$. However, by defining $\beta_T = \beta_{T,\mathrm{surf}} L$ where $\beta_{T,\mathrm{surf}}$ is the surface compressibility, using Eq. S19a, and setting $P_0 = 0$, one obtains

$$d\varepsilon_{xy} = -\frac{2\beta_{T,\mathrm{surf}}}{3\tau_P}\left(\gamma_0 - \left(\frac{\partial K}{\partial A} + \frac{\partial U}{\partial A}\right)\right) dt + \sqrt{\frac{4k_B T \beta_{T,\mathrm{surf}}}{3A\tau_P}} dW_{xy} \qquad \text{(S20)}$$

In practice, this means that in order to obtain a dynamics of the area $A$ with the correct relaxation time it is sufficient to:

- Set $\beta_{T,z} = 0$ so that $L$ does not vary during the simulation.
- Set $P_0 = 0$ to avoid an explicit dependence of the energy on the cell volume.
- Obtain an estimate of the area fluctuations $\sigma_A$ and estimate its compressibility as $\beta_{T,\mathrm{surf}} = \frac{\sigma_A^2}{\langle A\rangle k_B T}$.
- Set $\beta_{T,xy} = \beta_{T,\mathrm{surf}} L$, where $L$ is the fixed value of the cell height.

# Part II

# Supplementary results

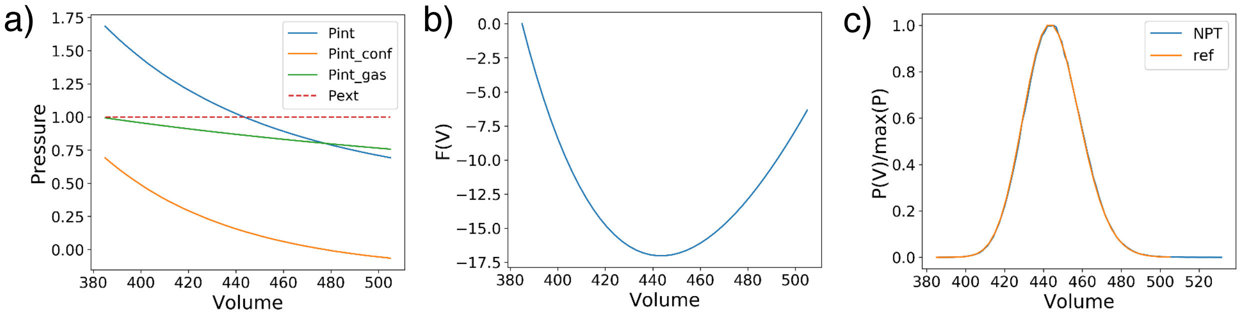


Supplementary Figure S1. Validation of the volume distribution obtained using stochastic cell rescaling barostat in the Lennard-Jones system. We first performed 41 simulations at constant volume, with volumes equally spaced in the range $[385, 505]$. For each simulation, we computed the configurational $(-\langle \frac{\partial U}{\partial V} \rangle)$ and kinetic $(\frac{Nk_BT}{V})$ contributions to the internal pressure $P_{\text{int}}$ (panel a). The free energy as a function of the volume $V$ was then obtained by thermodynamic integration as $F(V+\Delta V) = F(V) - \frac{P_{\text{int}}(V)+P_{\text{int}}(V+\Delta V)-P_{\text{ext}}(V)-P_{\text{ext}}(V+\Delta V)}{2}\Delta V$, with $\Delta V = 3$ (panel b). The probability distribution obtained from an $NPT$ simulation with stochastic cell rescaling, using $\tau_P = 1$ and the Euler integrator, can be compared with $P(V) \propto e^{-\frac{F(V)}{k_BT}}$ (panel c). The two distributions are undistinguishable.

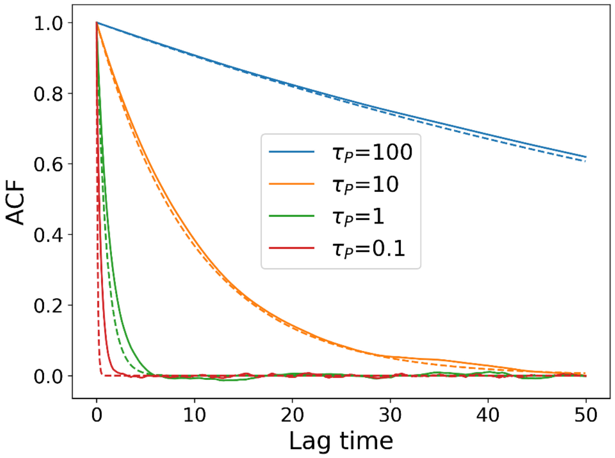


Supplementary Figure S2. Autocorrelation function (ACF) of the volume at varying $\tau_P$ values from simulations of the Lennard-Jones fluid. Results obtained using the Trotter-based integrator in the formulation with scaled momenta are displayed. Dashed lines represent exponentially decaying functions with the corresponding time constant ($e^{-\frac{t}{\tau_P}}$). For larger values of $\tau_P$ ($\tau_P = 10, 100$), the observed ACF are matching the exponential functions. For smaller values of $\tau_P$ ($\tau_P = 0.1, 1$) the observed decay is slower. This is due to the fact that in these simulations the bottleneck for volume sampling is the rearrangement of the atoms, which slows down the rearrangement given by first-order relaxation.

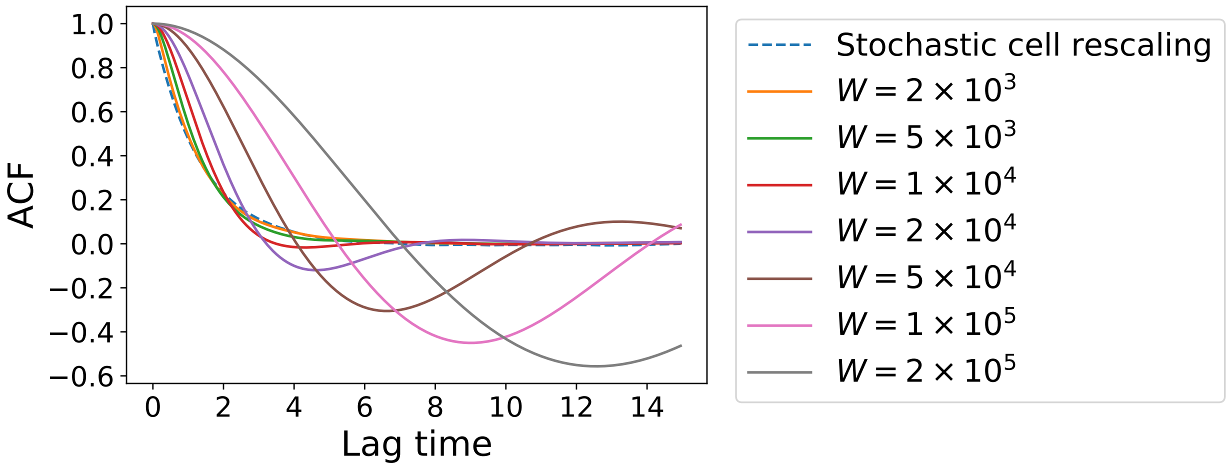


Supplementary Figure S3. Autocorrelation function (ACF) of the volume for a Langevin piston at varying barostat mass, obtained from simulations of the Lennard-Jones fluid. The Langevin piston is implemented by adding a Langevin thermostat on the barostat variable, using the barostat described in Ref. 1. $\tau_P$ is fixed to 1, and a range of values for the barostat mass $W$ is tested. The friction acting on the barostat velocity is defined as $\gamma(V) = \frac{9\tau_P V}{W\beta_T}$, as discussed in Section II. For a comparison, the autocorrelation function of a stochastic cell rescaling barostat with $\tau_P = 1$ is shown as a dashed line. When the piston mass is large, the autocorrelation function displays clear oscillations. When the piston mass is small enough, its behavior becomes very close to that of stochastic cell rescaling.

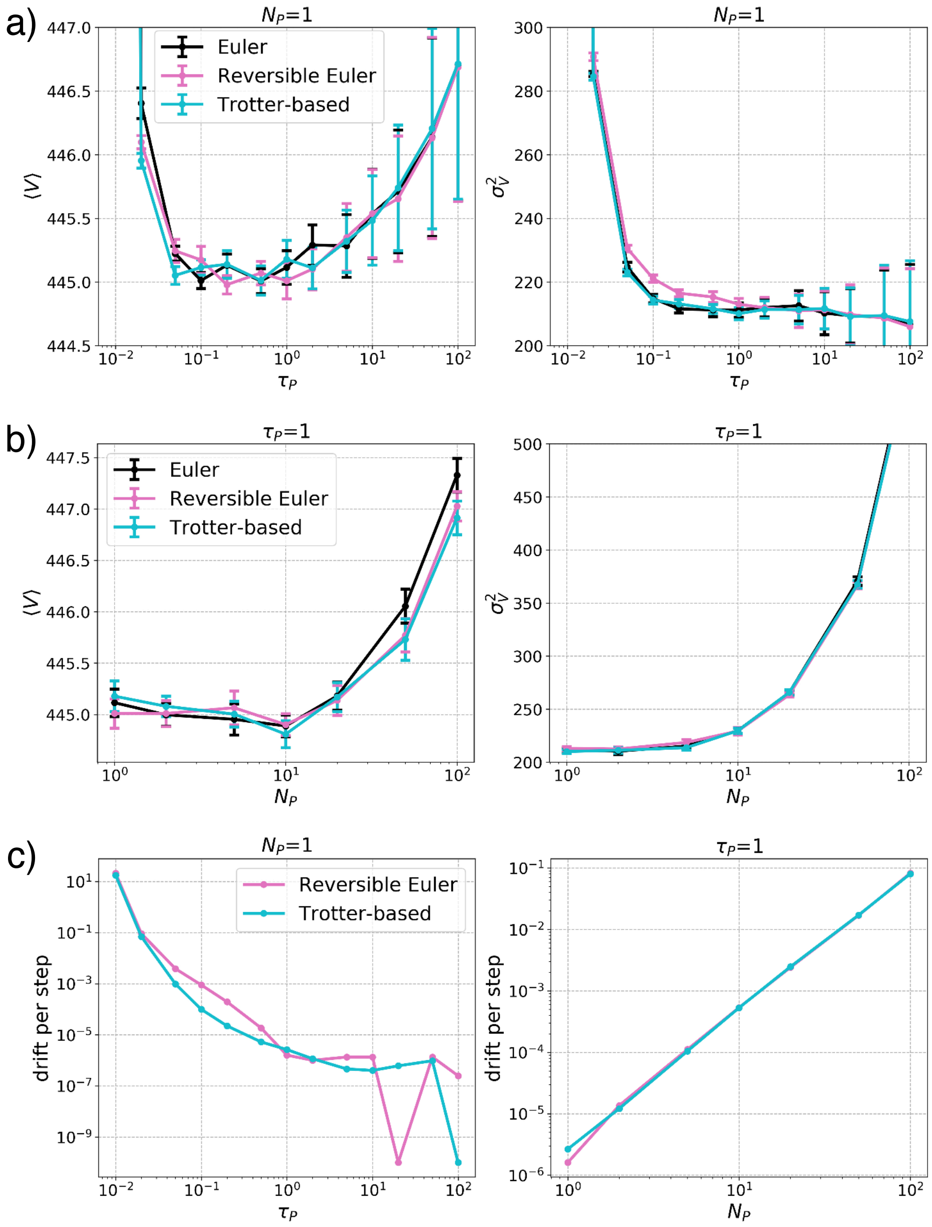


Supplementary Figure S4. Results from simulations of a Lennard-Jones fluid with the non-scaled momenta formulation of the integrators. a) Average and fluctuations of the volume (left and right panels, respectively) as a function of the time constant for pressure coupling ($\tau_P$) at fixed frequency for pressure coupling ($N_P =$ 1). b) Average and fluctuations of the volume (left and right panels, respectively) as a function of the frequency for pressure coupling ($N_P$) at fixed time constant for pressure coupling ($\tau_P = 1$). c) Effective energy drift per step, obtained from the slope of a line interpolating the effective energy drift on the entire trajectory. With some settings, a negative slope is obtained and is here shown as $10^{-10}$.

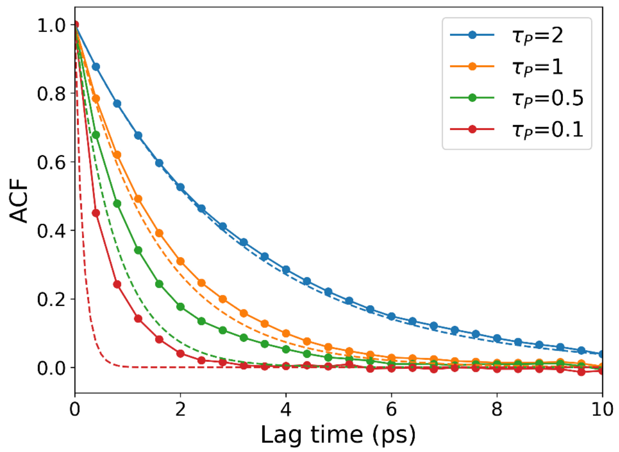


Supplementary Figure S5. Autocorrelation function (ACF) of the volume at varying $\tau_P$ values from simulations of the TIP3P water box in GROMACS. Results obtained using the C-rescale barostat are displayed. In this case, the estimate of the compressibility used as an input for the simulation ($\beta_{T,\mathrm{exp}} = 4.5 \times 10^{-5}\mathrm{bar}^{-1}$) does not correspond to the observed compressibility of TIP3P ($\beta_T \approx 6.3 \times 10^{-5}\mathrm{bar}^{-1}$). The volume is thus expected to relax on a modified timescale $\tau_P' = \frac{\beta_T}{\beta_{T,\mathrm{exp}}}$. Dashed lines represent exponentially decaying functions with the corresponding effective time constant ($e^{-\frac{t}{\tau_P'}}$). For the largest value of $\tau_P$ ($\tau_P = 2$), the observed ACF is matching the exponential function. For smaller values of $\tau_P$ ($\tau_P = 0.1, 0.5, 1$) the observed decay is slower. This is due to the fact that in these simulations the bottleneck for volume sampling is the rearrangement of the atoms, which slows down the rearrangement given by first-order relaxation.

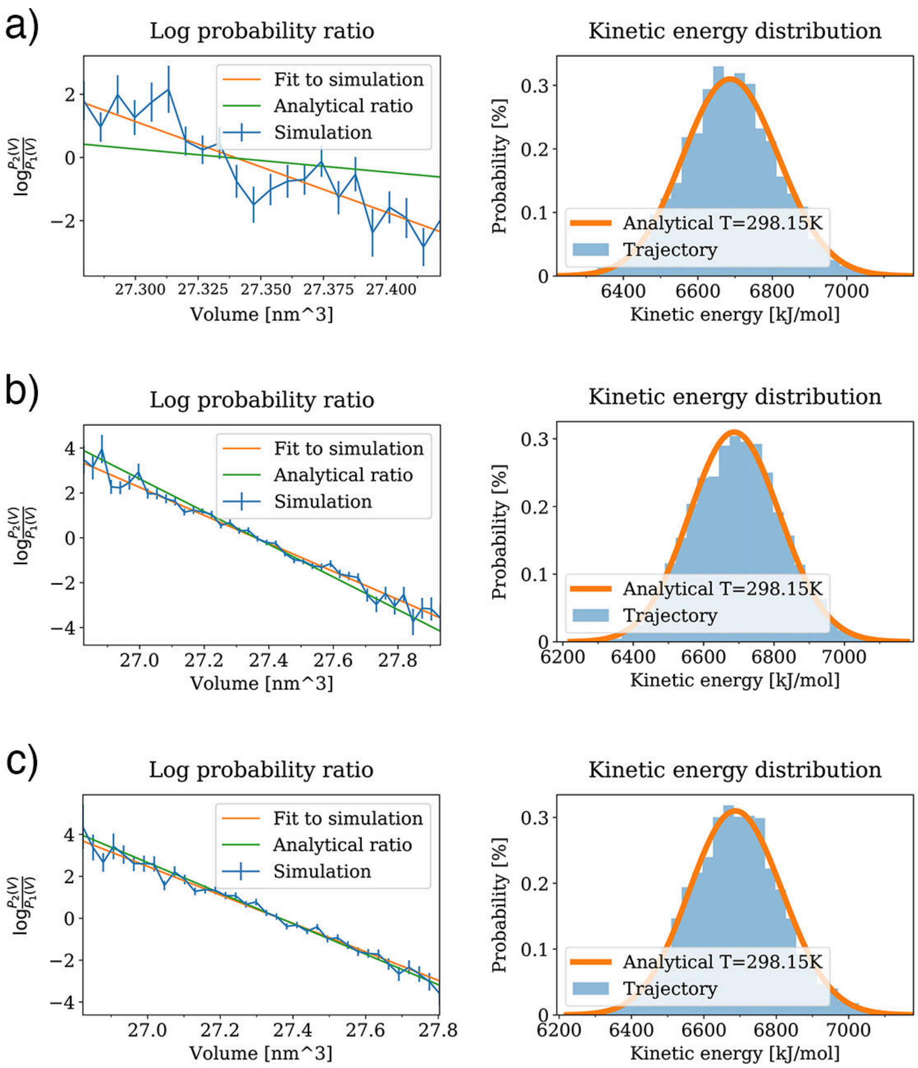


Supplementary Figure S6. Physical validation tests on a TIP3P water box with pressure coupling achieved through the a) Berendsen, b) Parrinello-Rahman and c) stochastic cell rescaling barostats. For the ensemble validation (left panels), two simulations were performed at a reference pressure of 1 bar and 301 bar, respectively. The simulation results at the lower and higher state points are used to calculate the ratio of the probability distribution of the volume (blue lines, with corresponding fitted lines in orange), and this ratio is then compared to the analytical expectation (green lines). The slopes of the fitted and the analytical lines are reported in Table S1. For the kinetic energy validation (right panels), the distribution of the kinetic energy in the lower state point (blue bars) is compared to the corresponding analytical reference (orange lines).

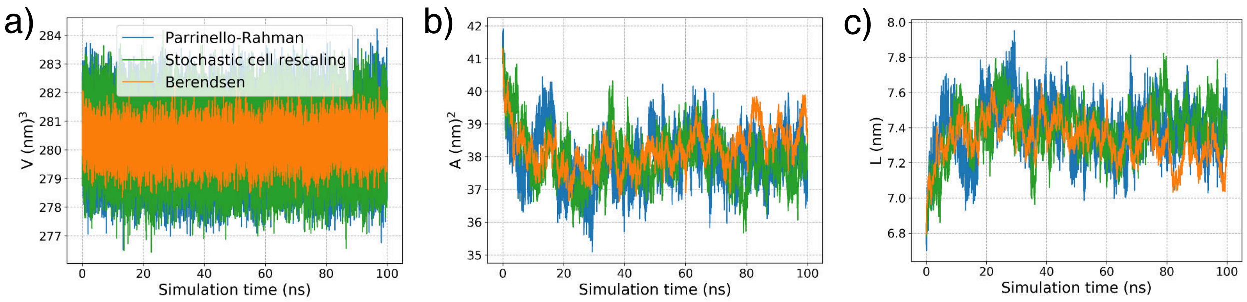


Supplementary Figure S7. Time series from the membrane system (KALP15 in DPPC) simulations. a) Volume, b) area of the simulation box in the *xy* plane, c) height of the simulation box along the z axis.

Supplementary Table S1. Slopes from the ensemble validation lines reported in figure S6. The slopes computed for the lines fitted on the simulation data are compared to the one of the analytical reference.

| | **Computed** | **Analytical expectation** |
|---|---|---|
| Berendsen | -32.36 ± 1.78 | -7.29 |
| Parrinello-Rahman | -6.35 ± 0.14 | -7.29 |
| Stochastic cell rescaling | -6.91 ± 0.18 | -7.29 |

## REFERENCES


[1] G. Bussi, T. Zykova-Timan, and M. Parrinello, "Isothermal-isobaric molecular dynamics using stochastic velocity rescaling," J. Chem. Phys. **130**, 074101 (2009).

[2] G. J. Martyna, D. J. Tobias, and M. L. Klein, "Constant pressure molecular dynamics algorithms," J. Chem. Phys. **101**, 4177–4189 (1994).

[3] P. Attard, "On the density of volume states in the isobaric ensemble," J. Chem. Phys. **103**, 9884–9885 (1995).

[4] S. E. Feller, Y. Zhang, R. W. Pastor, and B. R. Brooks, "Constant pressure molecular dynamics simulation: the Langevin piston method," J. Chem. Phys. **103**, 4613–4621 (1995).

[5] H. C. Andersen, "Molecular dynamics simulations at constant pressure and/or temperature," J. Chem. Phys. **72**, 2384–2393 (1980).

[6] D. Quigley and M. Probert, "Langevin dynamics in constant pressure extended systems," J. Chem. Phys. **120**, 11432–11441 (2004).

[7] S. Hottovy, A. McDaniel, G. Volpe, and J. Wehr, "The Smoluchowski-Kramers limit of stochastic differential equations with arbitrary state-dependent friction," Commun. Math. Phys **336**, 1259–1283 (2015).

[8] G. Bussi and M. Parrinello, "Accurate sampling using Langevin dynamics," Phys. Rev. E **75**, 056707 (2007).

[9] K.-H. Chow and D. M. Ferguson, "Isothermal-isobaric molecular dynamics simulations with Monte Carlo volume sampling," Comput. Phys. Commun. **91**, 283–289 (1995).

[10] J. Åqvist, P. Wennerström, M. Nervall, S. Bjelic, and B. O. Brandsdal, "Molecular dynamics simulations of water and biomolecules with a Monte Carlo constant pressure algorithm," Chem. Phys. Lett. **384**, 288–294 (2004).
